# Supplementary material for: High-precision spectroscopy of $^{20}$O benchmarking ab-initio calculations in light nuclei
Source: arXiv:2405.14305 source file (2024-05-23)
Supplement: Supplementary file 1 [file SupplementalMaterial.pdf]

# High-precision spectroscopy of $^{20}$O benchmarking *ab-initio* calculations in light nuclei. *Supplemental Material*


I. Zanon et al.[1,2]

[1] *INFN Laboratori Nazionali di Legnaro, Legnaro, Italy.*
[2] *Dipartimento di Fisica e Scienze della Terra, Università di Ferrara, Ferrara, Italy.*


## ADDITIONAL INFORMATION ON THE DATA ANALYSIS

The measurement was performed in triple coincidence with the VAMOS++ magnetic spectrometer for heavy ions detection, the MUGAST charged particle array and the AGATA $\gamma$ tracking array. From the proton spectroscopy in MUGAST, the excitation energy of the $^{20}$O recoil at the reaction point is determined. In the letter, the two dimensional correlation between the $\gamma$-rays decays in AGATA and the excitation energy, and the total projection of the tracked $\gamma$ ray spectrum are shown for $^{20}$O.

Figure 1 shows the projection of the two dimensional correlation on the excitation energy axis for $^{20}$O in coincidence with AGATA. The yrast $2^+_1$ and $4^+_1$ states and non-yrast $2^+_2$ and $3^+_1$ states are resolved. In brackets, tentative assignment for the $(2^+_3)$ and $(2^+_4)$ states at 5.0 MeV and 5.6 MeV respectively are indicated. A higher resolution spectrum and without requiring a prompt coincidence with AGATA was published in [1].

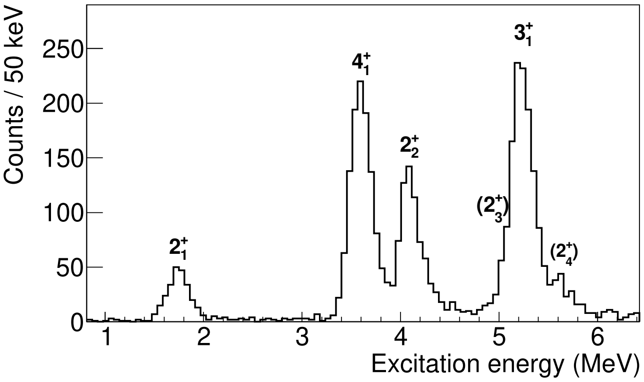


FIG. 1. Excitation energy spectrum measured in MUGAST for $^{20}$O in coincidence with AGATA.

The complete spectroscopic information of the gamma rays observed in the experiment is presented in Table I. In particular, the high energy resolution and the low background allowed for the observation, for the first time, of transitions in coincidence with the $(2^+_3)$ and $(2^+_4)$ states and a new transition at 1156.0(8) keV depopulating the $3^+_1$ state to the $2^+_2$ state. The presence of this transition is particularly relevant because it acts as a feeder, influencing the lifetime measurement of the $2^+_2$ state and introducing a systematic error if not taken into account.

TABLE I. Energies and lifetime of excited levels $J_i$ in $^{20}$O, corresponding transitions to final states $J_f$ and branching ratios (BR).

| $J_i$ | $E_X$ [MeV] | $\tau$ | $J_f$ | $E_\gamma$ [keV] | BR [%] |
|---|---|---|---|---|---|
| $2^+_1$ | 1.675(1) | 10.5(4) ps [2] | $0^+_1$ | 1674.5(4) | 100 |
| $4^+_1$ | 3.572(1) | | $2^+_1$ | 1897.7(3) | 100 |
| $2^+_2$ | 4.071(1) | 70(14) fs | $2^+_1$ | 2396.1(2) | 88(1) |
| | | | $0^+_1$ | 4071(1) | 12(1) |
| $(2^+_3)$ | 5.004(2) | | $2^+_1$ | 3329(2) | |
| $3^+_1$ | 5.228(1) | 54(12) fs | $2^+_2$ | 1156.0(8) | 28(1) |
| | | | $2^+_1$ | 3552.6(6) | 72(1) |
| $(2^+_4)$ | 5.629(5) | | $2^+_1$ | 3954(5) | |

## ADDITIONAL INFORMATION ON SIMULATION

The GEANT4 simulation used in this work used several inputs such as the geometry and response function of the apparatus, the reaction mechanism and the energy loss of the oxygen recoil into the gold backing used for the Doppler Shift Attenuation Method (DSAM) measurement. The geometry of AGATA and MUGAST, the measured intrinsic resolution of the AGATA detectors, as well as the uncertainties of particle and $\gamma$-ray energies and positions have been included to the simulation. For the reaction mechanism, the measured angular distributions of the excited states of $^{20}$O have been included in the simulation code. This is particularly important since the transferred momentum $L$ defines the velocity distribution of each excited state. The measured velocity distributions of the $^{20}$O recoils at the reaction vertex deduced from two-body kinematics using the measured proton energy and angle in MUGAST for the $2^+_1$, $4^+_1$, $2^+_2$ and $3^+_1$ states is shown in the Figure 2. We underline that the velocity distribution ($\beta$ = v/c) is therefore constrained by the experimental setup for each state under investigation at the reaction point in the $CD_2$ target.

Another key ingredient of the simulation is the control of the slowing down process into the Au backing foil placed after the $CD_2$ target where the Doppler Shift Attenuation Method is used to determined the nuclear

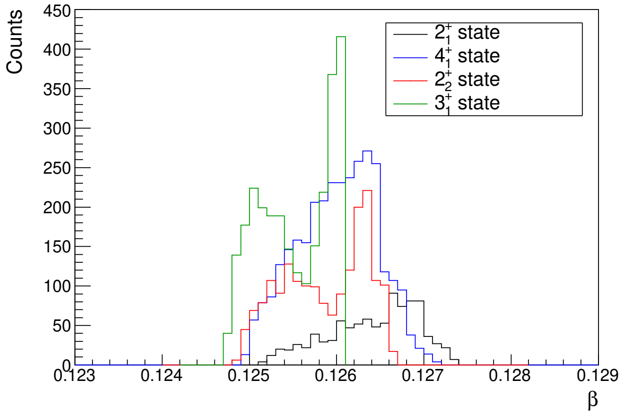


FIG. 2. Measured velocity ($\beta$ = v/c) distribution at the reaction point for the different excited states of $^{20}$O

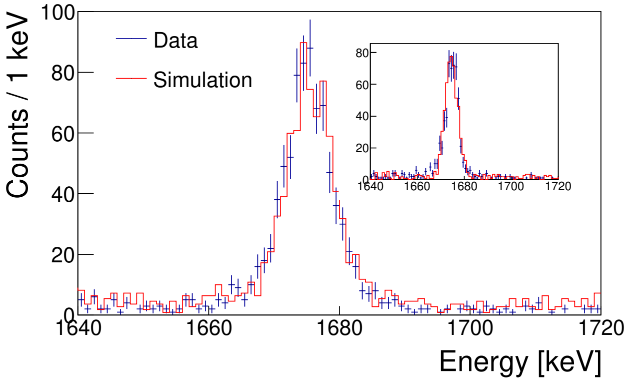


FIG. 4. (Color online) Comparison between experimental data (blue) and simulation (red) for the Doppler-corrected $2_1^+ \to 0_1^+$ transition at 1675 keV in $^{20}$O using the $CD_2$+Au target. In the inset, the same spectra using the $CD_2$ target.

lifetime. The oxygen stopping power in gold was constrained in our GEANT4 simulation by the available data [3] and verified using SRIM [4] and LISE++ [5] softwares. The compilation is shown in Figure 3. The GEANT4 outputs are shown in blue in the Figure with a good agreement with the measurement and models in the range of energy of the $^{20}$O recoil. The 10% difference at 10 MeV/u has no influence on the final result and the fluctuation remains below the statistical error.

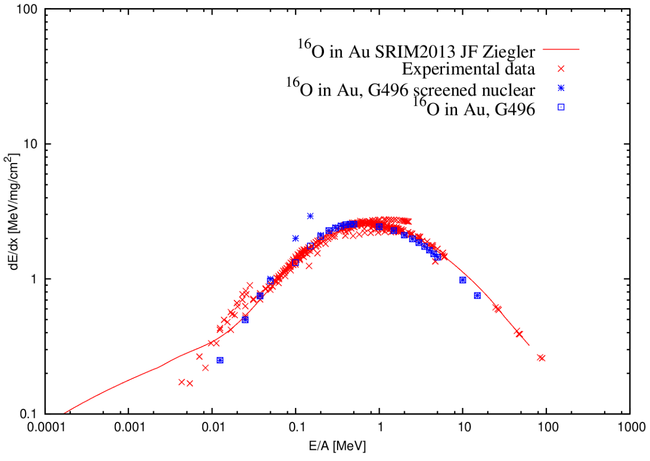


FIG. 3. (Color online) Experimental and calculated stopping-power of oxygen in gold as function of kinetic energy.

The simulation was validated using the spectroscopy of the $2_1^+$ state in $^{20}$O at 1675 keV. In this experiment, most of the decays of states with a lifetime longer than few ps occur after the Au backing. For states with a lifetime shorter than $10^{-2}$ fs, all decays occur in the $CD_2$ target and are not subject to Doppler broadening connected to lifetime effects. The simulation was first benchmarked by comparing the experimental and simulated spectra for the decay of the $2_1^+$ excited state, obtained using the $CD_2$ target. The simulation used the $2_1^+$ energy and its known lifetime $\tau$=10.5(4)ps [2] as an input. The inset of Fig. 4 shows the detected energies of the 1675-keV $2_1^+ \to 0_1^+$ $\gamma$-ray transition in blue and the corresponding simulation in red after Doppler correction. The measured and simulated energies of the transition are 1674.6(2) keV and 1674.5(2) keV, respectively. The measured Full Width Half Maximum (FWHM) is 6.5(3) keV to be compared to the simulated value 6.2(2) keV. The agreement is very good and validates the geometry and response function. Additionally, Fig. 4 shows the spectra obtained using the $CD_2$+Au target. The event-by-event Doppler-correction includes a calculated energy loss in the Au backing validated in Figure 3 to reproduce the energy of the transition at rest. By comparing the experimental and simulated $2_1^+ \to 0_1^+$ transition spectra, the energy loss process in the gold material and thickness of the gold foil with respect to the nominal value were validated in the simulation. The measured and simulated energies are 1675.1(2) keV and 1675.5(2) keV, respectively. The measured FHWM is 9.2(4) keV to be compared to the simulated value 8.7(3) keV.

## ADDITIONAL INFORMATION ON THE LIFETIME MEASUREMENT

The nuclear lifetimes using the DSAM method are extracted from the simulation using as degrees of freedom the energy of the $\gamma$-ray transition at rest and the lifetime of the excited state using the least-$\chi^2$ method. The simulations were performed varying the energy of the transition at rest from 2394 keV to 2398 keV and the lifetime of the $2_2^+$ state from 40 fs to 175 fs. For the analysis, the least-$\chi^2$ method, performed using the Neyman's formula [6], was employed after re-binning the experimental histogram by requiring at least 10 events per bin,

ensuring the gaussian approximation for error estimation. The statistical errors were estimated by requiring $\chi^2 - \chi^2_{\rm min} = \Delta\chi^2 = 2.3$ (4.6) for a 68% (90%) confidence limit [7]. Figure 5 shows the two dimensional $\chi^2$ surface for the $2_2^+$ state lifetime. The x-axis is the energy at rest of the $2_2^+ \rightarrow 2_2^+$ transition and the y-axis is the lifetime of the $2_2^+$ state set in the simulation. The z-axis represents the corresponding $\chi^2$ surface. It is used to determine the value of the nuclear lifetime corresponding to the minimum $\chi^2$ value and the corresponding error bars as given in the letter.

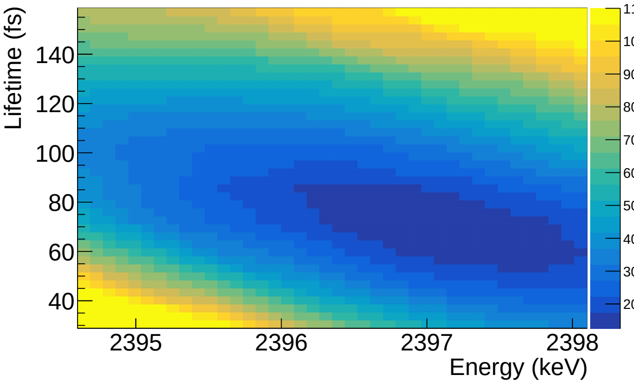


FIG. 5. (Color online) Two dimensional $\chi^2$ surface for the $2_2^+$ state lifetime.

## ADDITIONAL INFORMATION ON THE DISCUSSION FOR $^{19}$O

The level scheme of $^{19}$O was also computed for the three different Hamiltonians in the *ab-initio* VS-IMSRG calculations and USDB shell model and compared to the experimental data as presented in Figure 7. The goal is to demonstrate the consistency of the present calculation between $^{20}$O and its $^{19}$O core. Particular interest was in the agreement with the $1/2_1^+$ state in $^{19}$O interpreted as the single particle excited state with the $(d_{5/2})^2(s_{1/2})^1$ configuration. The best agreement for the *ab-initio* VS-IMSRG calculations is obtained for the 1.8/2.0(EM) Hamiltonian's with the proper sequence of $5/2^+$, $3/2^+$, $1/2^+$ and $9/2^+$ states.

The consistency between $^{19}$O and $^{20}$O is shown in figure 6. It shows the correlation between the $1/2^+$ state excitation energy in $^{19}$O and the difference in excitation energy between the $2_1^+$ and $2_2^+$ states in $^{20}$O for the three different Hamiltonian's and the experimental data. Even though the agreement for the difference in energy between the $2^+$ states with the data is quite convincing, the 1/2+ state in $^{19}$O is overestimated by half MeV.

Finally, table II shows the dominant configurations for

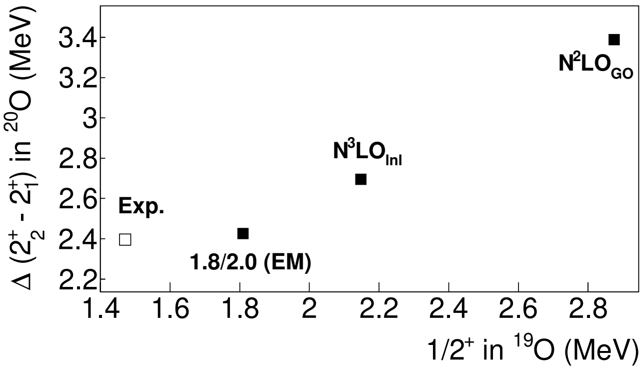


FIG. 6. Correlation between the excitation energy of the $1/2^+$ state in $^{19}$O and the difference between the $2_1^+$ and $2_2^+$ states in $^{20}$O for the three different Hamiltonian's and the experimental data.

the $0_1^+$, $2_1^+$ ($5/2_1^+$) states in $^{20}$O ($^{19}$O) and the single neutron $2_2^+$, $3_1^+$ ($1/2_1^+$) excited states ($d_{5/2} \rightarrow (s_{1/2})^{+1}$) in $^{20}$O ($^{19}$O), respectively, for *ab-initio* VS-IMSRG calculations employing three different Hamiltonians.

This material is used to demonstrate that the present *ab-initio* calculations can be used for microscopical description of excited states in exotic nuclei giving reasonable agreement with the data similarly to the conventional phenomenological shell-model approaches.


[1] M. Assié *et al.*, Nucl. Instr. and Meth. A **1014**, 165743 (2021).
[2] P. Raghavan, Atomic Data and Nuclear Data Tables **42**, 189 (1989).
[3] "https://www-nds.iaea.org/stopping/," AIEA.
[4] J. F. Ziegler and J. P. Biersack, "The stopping and range of ions in matter," in *Treatise on Heavy-Ion Science: Volume 6: Astrophysics, Chemistry, and Condensed Matter* (Springer US, Boston, MA, 1985) pp. 93–129.
[5] O. Tarasov and D. Bazin, Nucl. Instr. and Meth. B **266**, 4657 (2008).
[6] S. Baker and R. Cousins, Nucl. Instr. and Meth. **221**, 437 (1984).
[7] Particle Data Group *et al.*, Progress of Theoretical and Experimental Physics **2020** (2020).

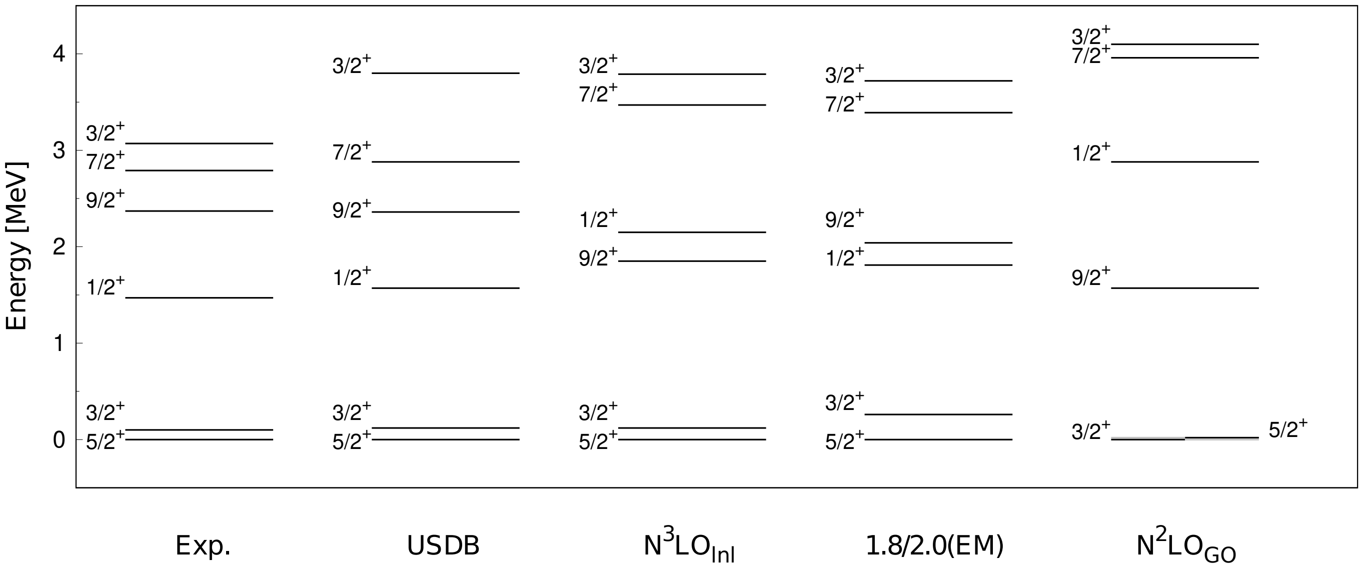


FIG. 7. Experimental $^{19}$O excited states compared to theoretical USDB shell-model calculations and VS-IMSRG results obtained with three different Hamiltonians.

| | $^{20}$O | | | | $^{19}$O | |
|---|---|---|---|---|---|---|
| | $0_1^+$ | $2_1^+$ | $2_2^+$ | $3_1^+$ | $5/2_1^+$ | $1/2_1^+$ |
| | | | N$^3$LO$_{lnl}$ | | | |
| $0d_{5/2}$ | 3.72 | 3.73 | 2.92 | 2.92 | 2.86 | 1.94 |
| $1s_{1/2}$ | 0.14 | 0.18 | 1.01 | 1.00 | 0.07 | 1.00 |
| $0d_{3/2}$ | 0.14 | 0.09 | 0.06 | 0.09 | 0.07 | 0.06 |
| | | | 1.8/2.0 (EM) | | | |
| $0d_{5/2}$ | 3.69 | 3.70 | 2.94 | 2.92 | 2.85 | 1.94 |
| $1s_{1/2}$ | 0.17 | 0.20 | 0.99 | 1.00 | 0.09 | 1.00 |
| $0d_{3/2}$ | 0.14 | 0.09 | 0.06 | 0.09 | 0.07 | 0.07 |
| | | | N$^2$LO$_{GO}$ | | | |
| $0d_{5/2}$ | 3.82 | 3.81 | 2.93 | 2.93 | 2.90 | 1.95 |
| $1s_{1/2}$ | 0.08 | 0.12 | 1.02 | 1.00 | 0.04 | 1.00 |
| $0d_{3/2}$ | 0.11 | 0.07 | 0.05 | 0.07 | 0.05 | 0.05 |

TABLE II. Occupancy of the neutron orbitals for $2_1^+$ and $2_2^+$ states in $^{20}$O nucleus and $9/2_1^+$ and $1/2_1^+$ states in $^{19}$O for *ab-initio* VS-IMSRG calculations employing three different Hamiltonians.
